# Supplementary material for: Analysis of nanometre sized aligned conical pores using SAXS
Source: arXiv:1909.10665 source file (2020-07-05)
Supplement: Supplementary file 1 [file SupplementaryAH.pdf]

## CONE ROTATION ABOUT ONE AXIS

In Fig. 1(a), a three dimensional cone is shown aligned with the Y axis of a three dimensional coordinate system with the cone apex at the origin. In our experimental set-up this corresponds to a rotation from the aligned position (coaxial with the Z axis) about the X axis by 90°. In the experimental set-up the plane of the detector is parallel to the XY plane. In Fig. 1(b), the cone is rotated around the X axis by an angle $\gamma$. The axis of the cone is represented by the vector shown in blue ($\vec{H}$). The projection of the axis of the cone onto the Y axis is shown in red, as $\vec{H}(y)$. In both figures the 3-D cone is viewed normal to the XY plane along the Z axis on the left, and from the side along the X axis on the right.

In Fig. 1(a) where the axis of the cone is aligned with the Y axis, the geometric projection of $\vec{H}$ onto the Y axis is equal to $\vec{H}$, and the half cone opening angle $\beta$ projected onto the XY plane is $\beta$. In Fig. 1(b) where the cone is rotated, the geometric projection of the cone axis $\vec{H}$ is given by $\vec{\mathrm{H}}(\mathrm{y}) = \vec{\mathrm{H}}\sin\gamma$.

The parameters of a cone with a half opening angle $\beta$, base radius $R_0$ and height $H$ are related by Equation 1:

$$\tan\beta = \frac{R_0}{H} \tag{1}$$

When the cone is rotated as shown in Figs. 1(b) the projected base radius of the cone does not change due to the rotation ($R_0 = R_0$). The half cone opening angle projected onto the XY plane is equivalent to the angle observed between the streaks on the SAXS scattering images, $\phi$. The projected cone parameters are shown by the triangle at the lower centre of Fig. 1(b), and are related by:

$$\tan\phi = \frac{R_0}{\vec{H}(y)} \tag{2}$$

Since $\vec{\mathrm{H}}(\mathrm{y}) = \vec{\mathrm{H}}\sin\gamma$, substitution of the expression for $R_0$ from Equation 1 gives the relationship between the three angles $\phi$, $\beta$ and $\gamma$:

$$\tan\phi = \frac{\tan\beta}{\sin\gamma} \tag{3}$$

## SIMULATION

To study the effect of rotation of the physical cones in two directions, a video simulation was made (see Figure 2, and the video Supplementary_AH_SD.mp4, at URLXXXX). In the video a 3-D drawing of a physical cone is shown on the left. On the right simulated scattering intensity patterns are shown which correspond to the position of the real space cones as they are rotated with respect to the x-ray beam. The scattering intensity images were simulated using Equation 10 (rotation by the angle $\gamma$). Rotation by the angle $\xi$ was implemented by applying a rotation matrix to equations 11(a)-(c), representing a rotation around the Y axis by the angle $\xi$.

In the video the cone is first rotated by an angle $\gamma$, from $\gamma$=0° to 90°. It then rotates back to $\gamma = 30°$ and $\gamma$ is fixed while $\xi$ is rotated from 0 to 30°. $\gamma$ and $\xi$ are then both decreased at the same rate from 30° to 0°.

## FIGURES

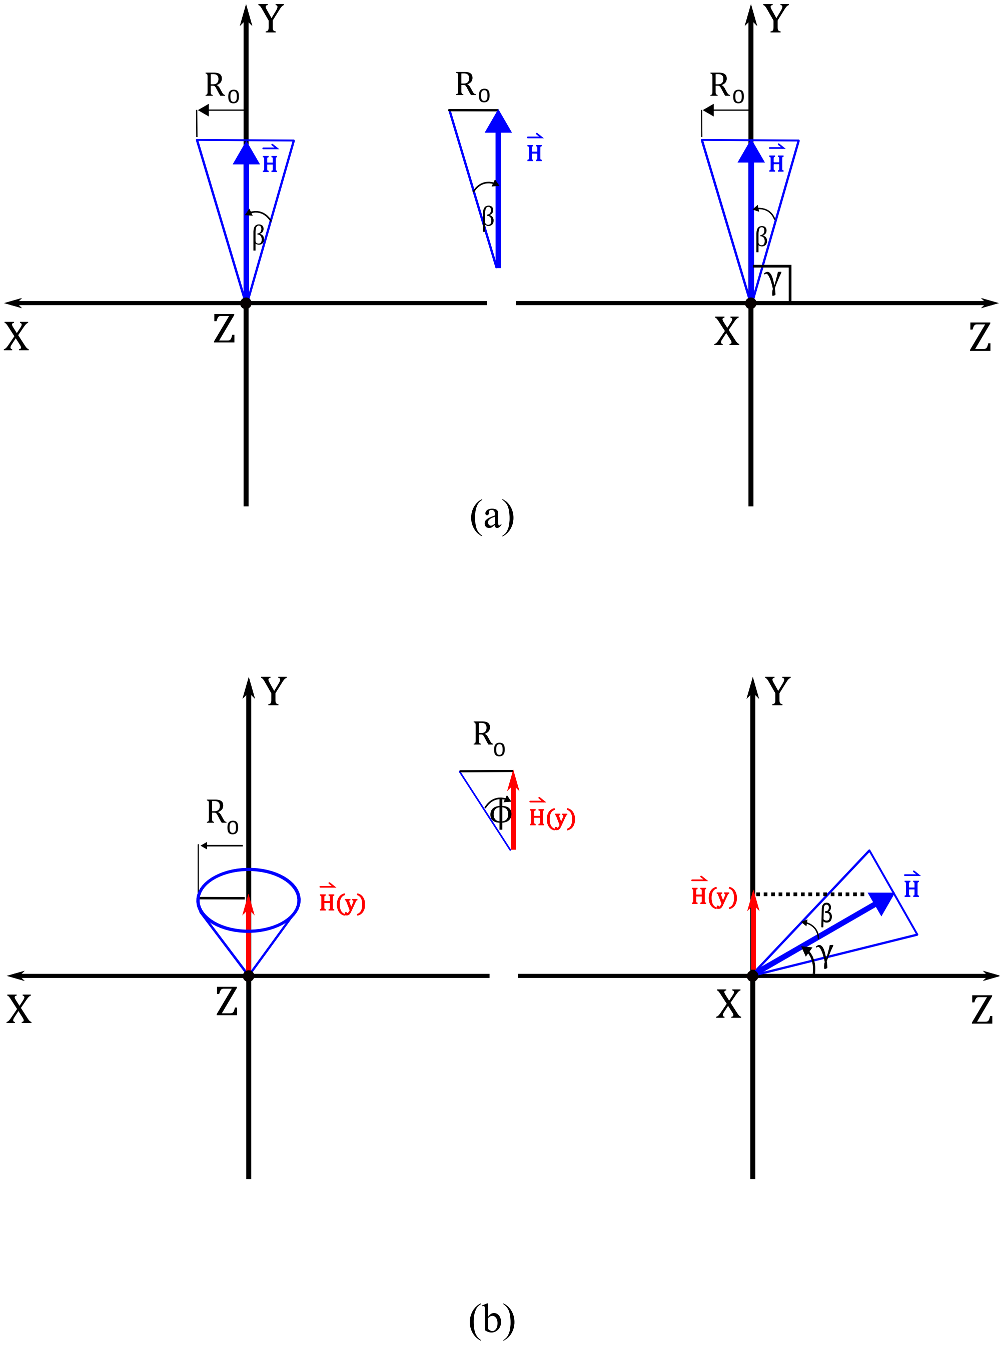


FIG. 1. Rotation of cone about the X axis. (Not to scale.)

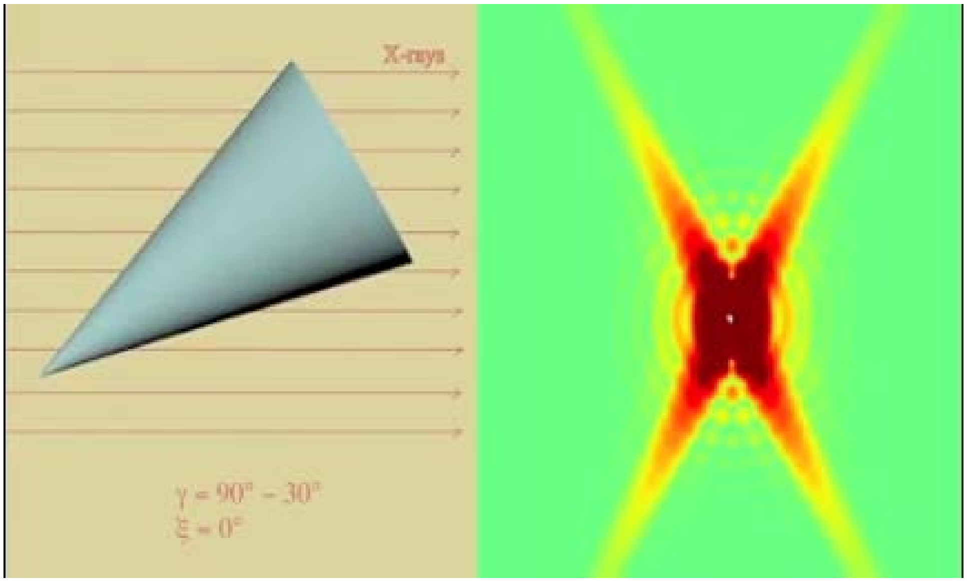


FIG. 2. Animation of 2-D scattering simulations showing the effect of tilting the cones by an angle $\gamma$ around the X axis, followed by a rotation of $\xi$ around the Y axis (see the video Supplementary_AH_SD.mp4, at URLXXXX).
